# Supplementary material for: Spatio-Temporal Meta Contrastive Learning
Source: arXiv:2310.17678 source file (2023-10-26)
Supplement: Supplementary file 1 [file supplementary.tex]

\section{Supplementary Material}
\balance
\label{sec:supplementary}
